# Supplementary material for: HRMOS: A High-Resolution Multi-Object Spectrograph for the VLT
Source: arXiv:2607.04916 source file (2026-07-06)
Supplement: Supplementary file 1 [file appendix.tex]

\fancyhead[R]{Ch. \thechapter. \textsf{Appendix}}

\section{Estimating the precision in abundances and abundance ratios}

In this appendix, we report the estimated uncertainties on the derived abundances of various elements
and isotopic ratios as a function of the expected abundance, signal-to-noise ratio (SNR), and surface gravity 
in spectra typical of HRMOS-like instruments. The errors were evaluated using synthetic spectra 
covering a wide range of stellar parameters representative of our survey targets, taking into account 
both photon noise and continuum placement uncertainties.

Figure~\ref{fig:th_precision} illustrates the dependence of the abundance uncertainty on the intrinsic 
abundance and SNR for [Th/Fe], adopting the following stellar parameters: $T_{\mathrm{eff}}$--log~$g$ 
pairs of 5800~K--3.7~dex, 6400~K--4.1~dex, and 6000~K--4.5~dex for dwarf main-sequence stars, and 
4800~K--1.2~dex, 5000~K--2.0~dex, and 5200~K--2.5~dex for red giant branch stars. Microturbulence 
values of $v_{\rm mic} = 1.2$~km\,s$^{-1}$ and 2.0~km\,s$^{-1}$ were adopted for dwarfs and giants, 
respectively.

In a similar manner, Figures~\ref{fig:origin_la_precision}, \ref{fig:origin_eu_precision}, and 
\ref{fig:origin_pb_precision} show the uncertainties in the abundance ratios [La/Fe], [Eu/Fe], and [Pb/Fe], 
respectively. Finally, Figure~\ref{fig:origin_ba_precision} presents the estimated errors on the isotopic 
fractions of Ba.

These results provide a quantitative guide to the achievable precision in chemical abundance studies 
across different stellar populations observed with HRMOS-class instruments, and are particularly 
useful for planning high-resolution multi-object spectroscopic surveys and for interpreting detailed 
chemical patterns in stars of varying evolutionary stages.

\begin{figure}[h]
\centering
    \includegraphics[width=0.24\linewidth]{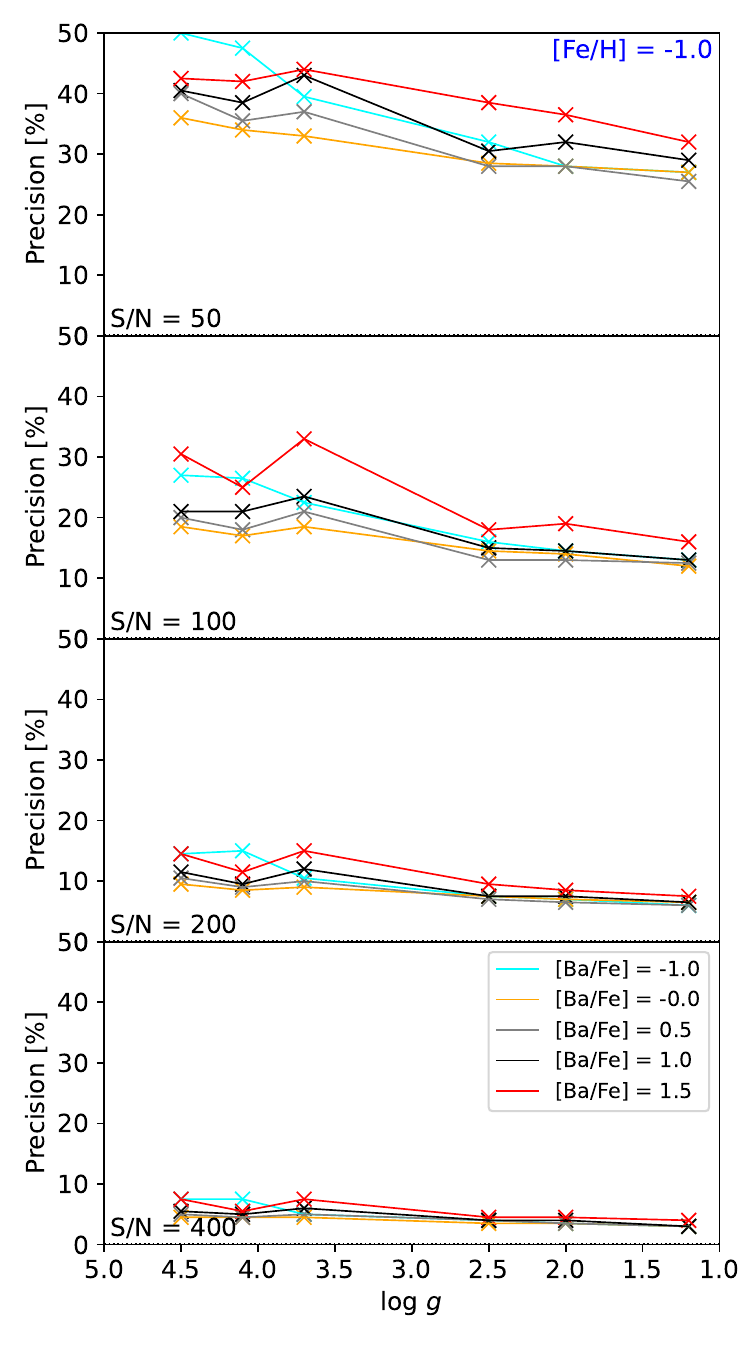} 
   \includegraphics[width=0.24\linewidth]{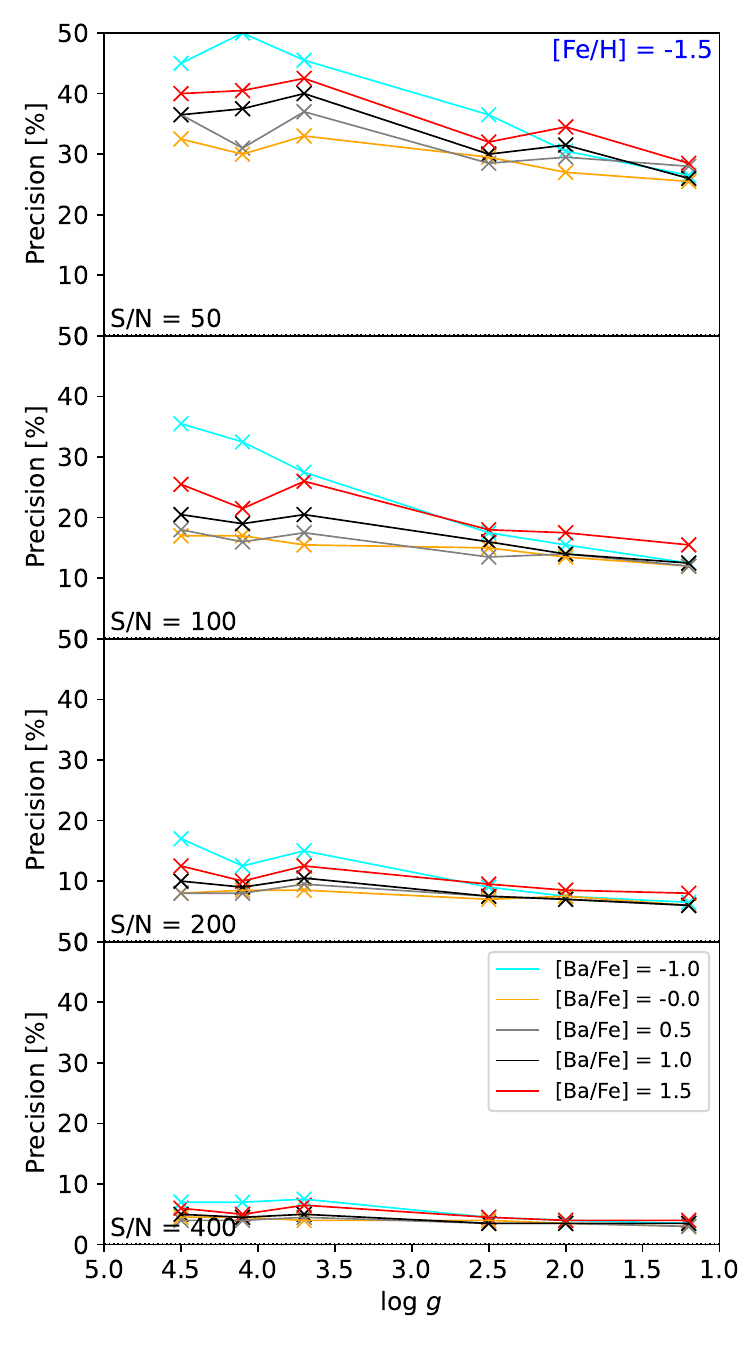} 
   \includegraphics[width=0.24\linewidth]{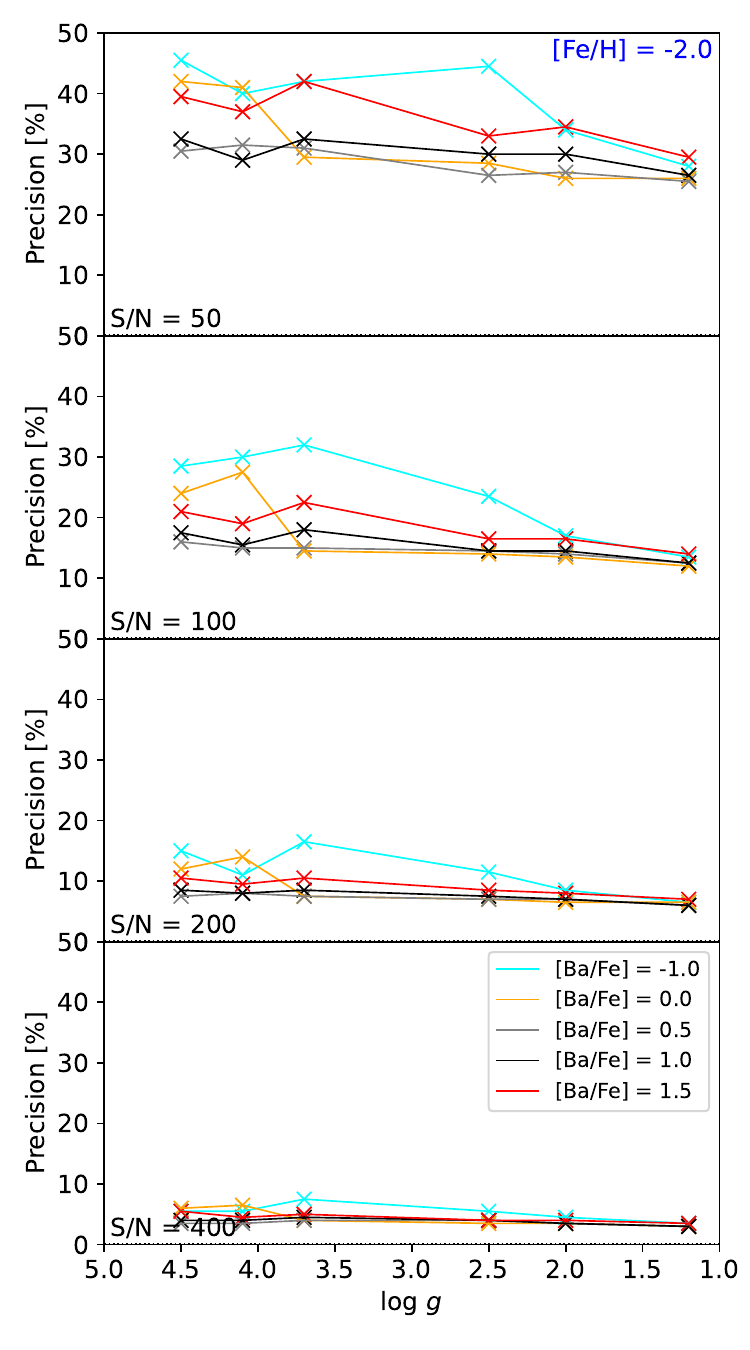} 
   \includegraphics[width=0.24\linewidth]{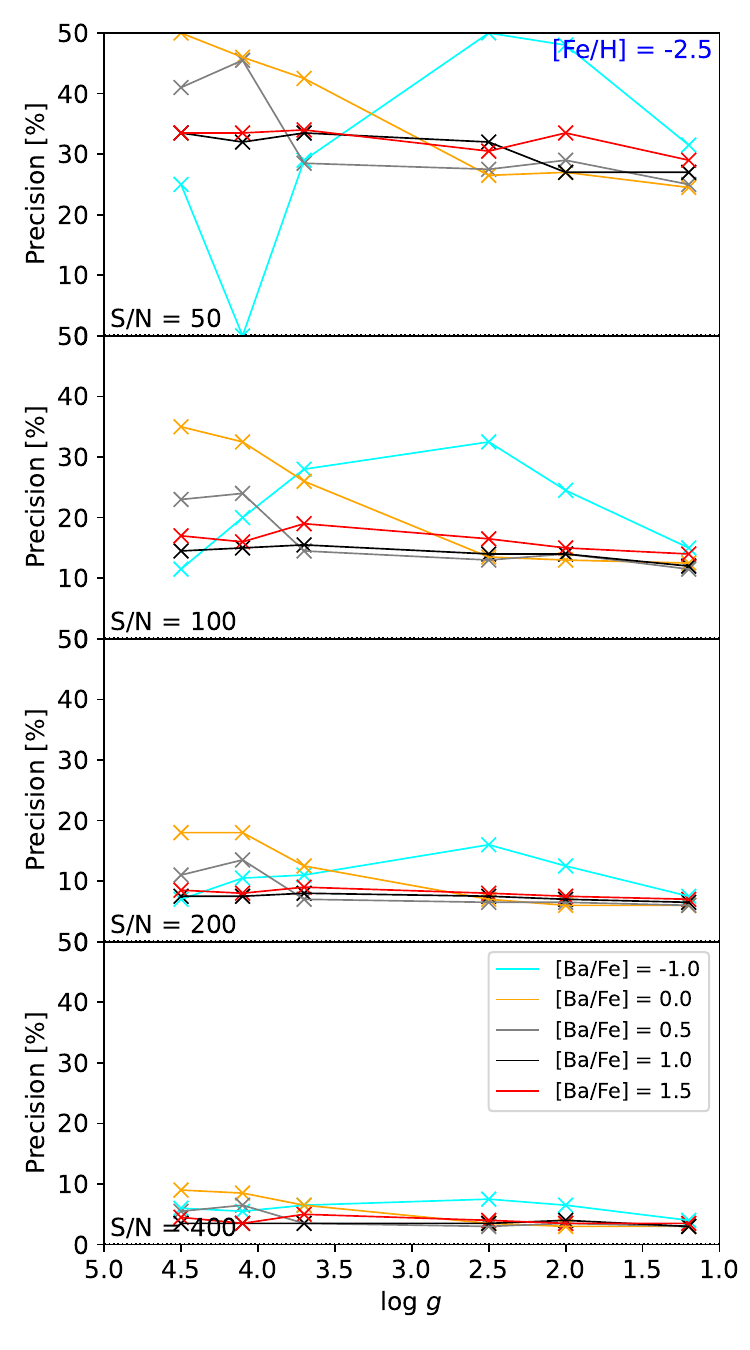}   
    \caption{Precision in the measurement of Th abundances as a function of metallicity and of SNR. The adopted stellar parameters are the $T_{\mathrm{eff}}$-log~$g$ pairs of 5800~K-3.7~dex, 6400\,K-4.1\,dex, and 6000\,K-4.5\,dex for dwarf main sequence stars, and 4800\,K-1.2\,dex, 5000\,K-2.0\,dex, and 5200\,K-2.5\,dex for the red giant branch stars. For dwarfs and giants, microturbulence values of $v_{mic} = 1.2$ and $2.0$~km\,s$^{-1}$, respectively, are assumed. }
    \label{fig:th_precision}
\end{figure}

\begin{figure}
\centering
    \includegraphics[width=0.24\linewidth]{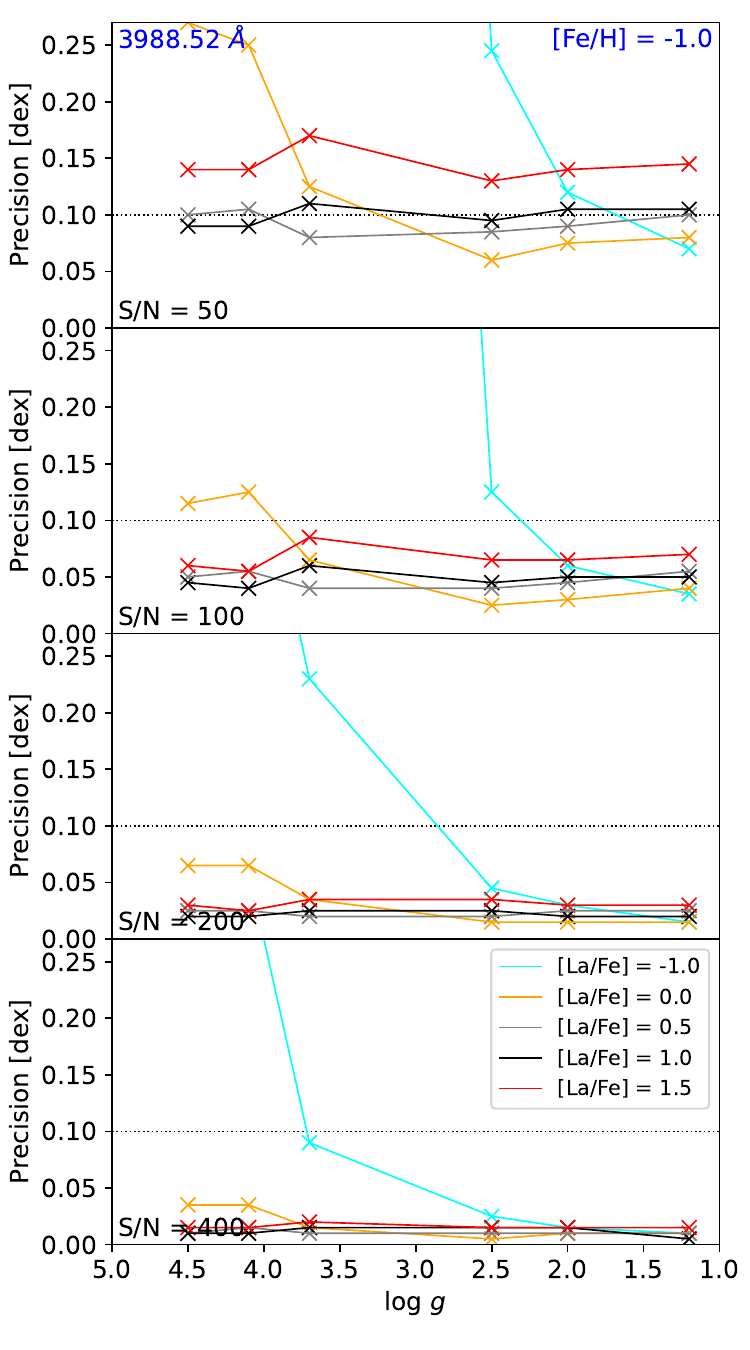} 
    \includegraphics[width=0.24\linewidth]{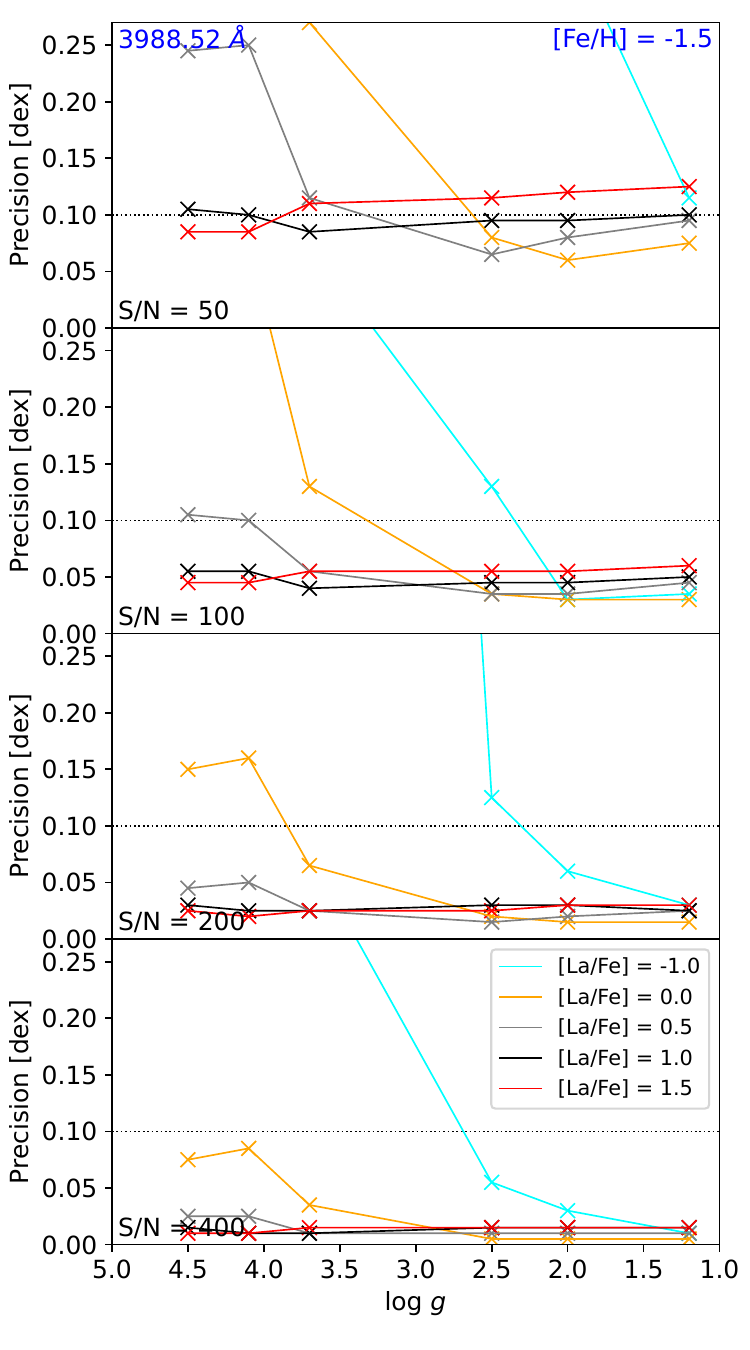} 
   \includegraphics[width=0.24\linewidth]{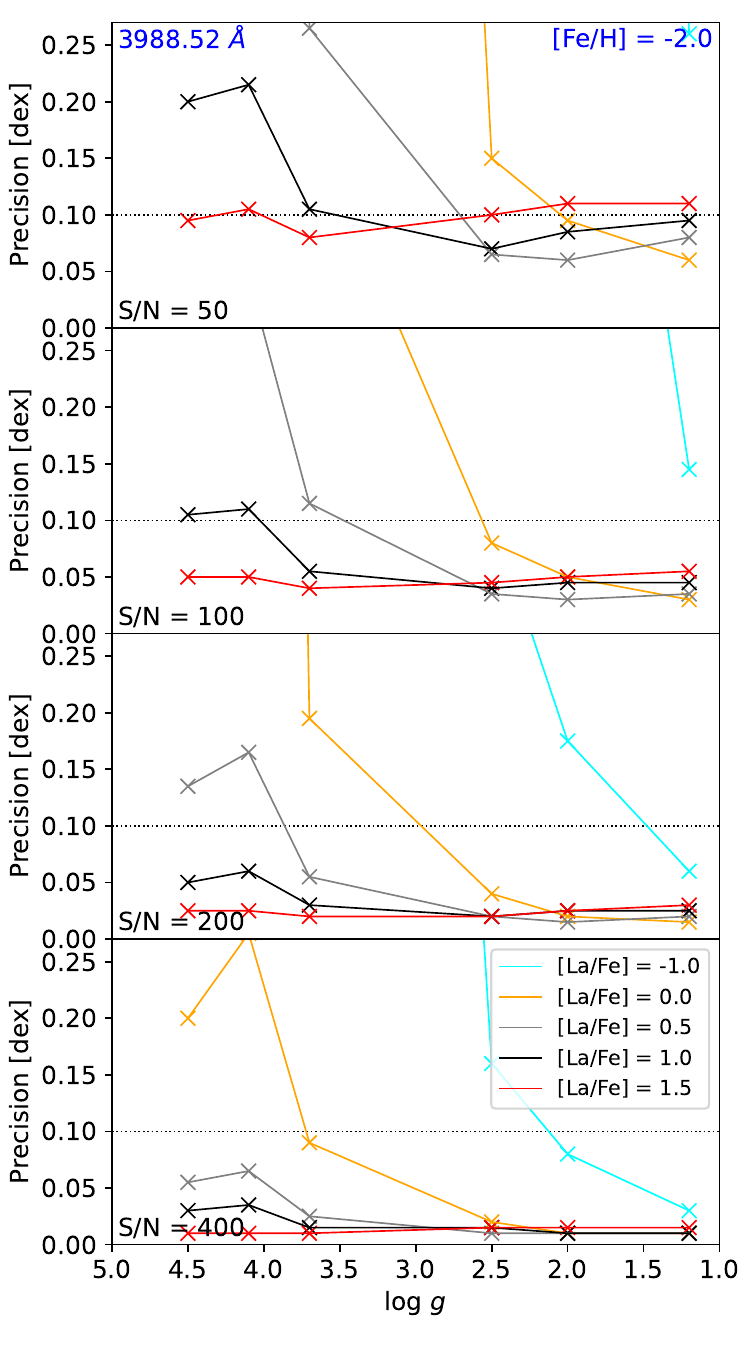} 
   \includegraphics[width=0.24\linewidth]{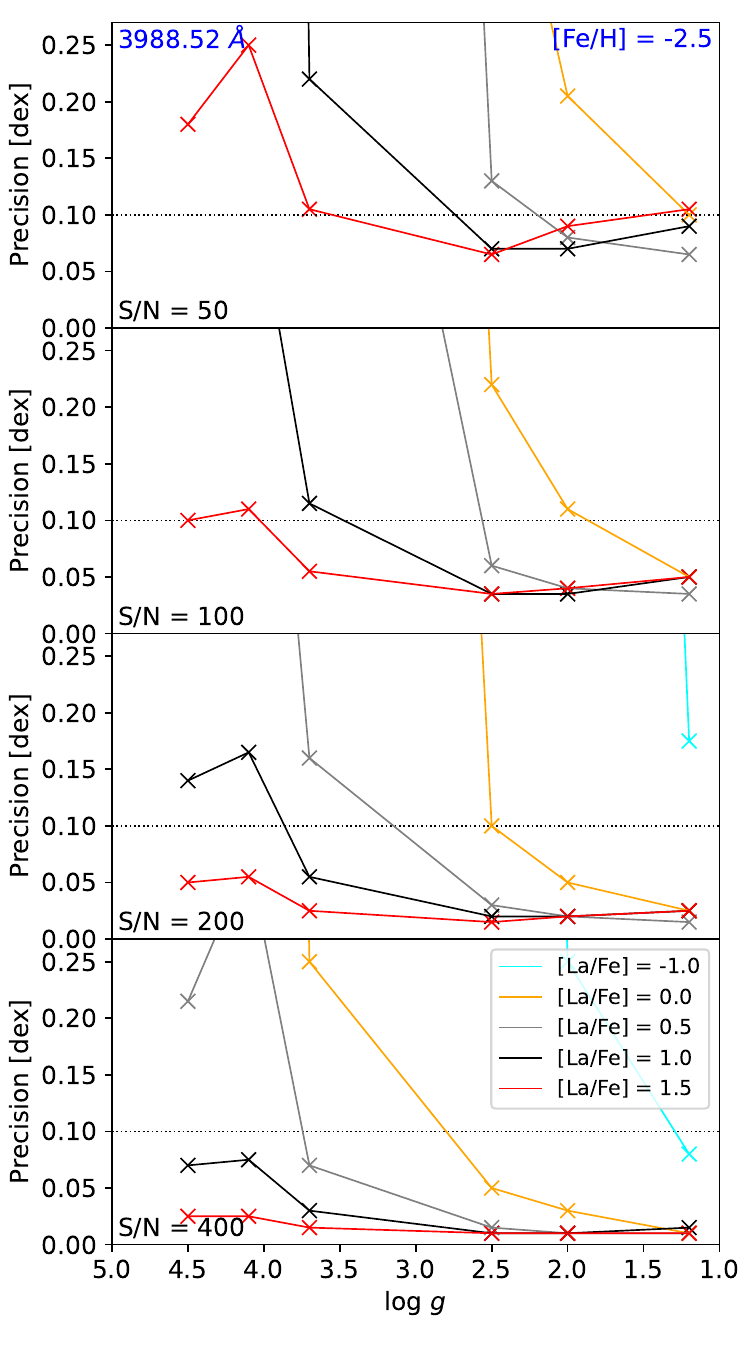}   
    \caption{Precision in the measurement of La abundances as a function of metallicity and of SNR. Stellar parameters are as in Fig.~\ref{fig:th_precision}. }
    \label{fig:origin_la_precision}
\end{figure}

\begin{figure}
\centering
    \includegraphics[width=0.24\linewidth]{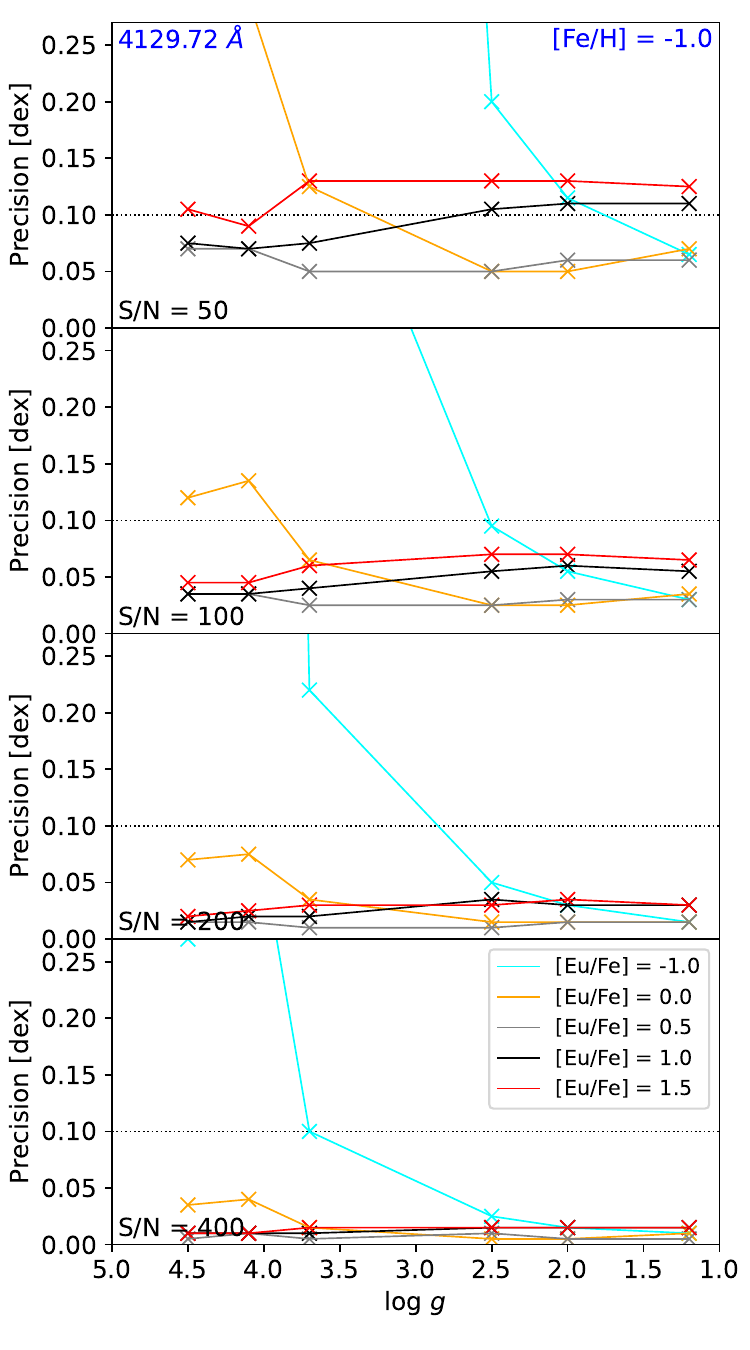} 
    \includegraphics[width=0.24\linewidth]{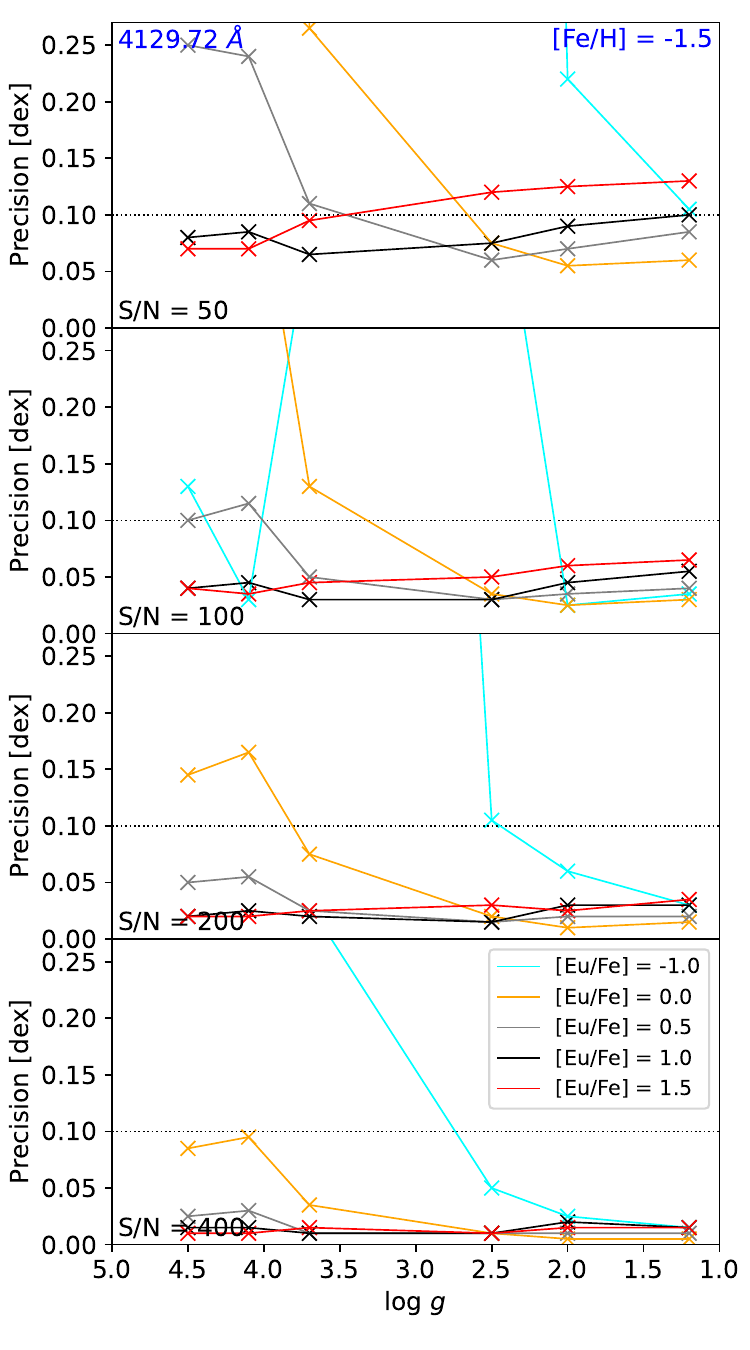} 
   \includegraphics[width=0.24\linewidth]{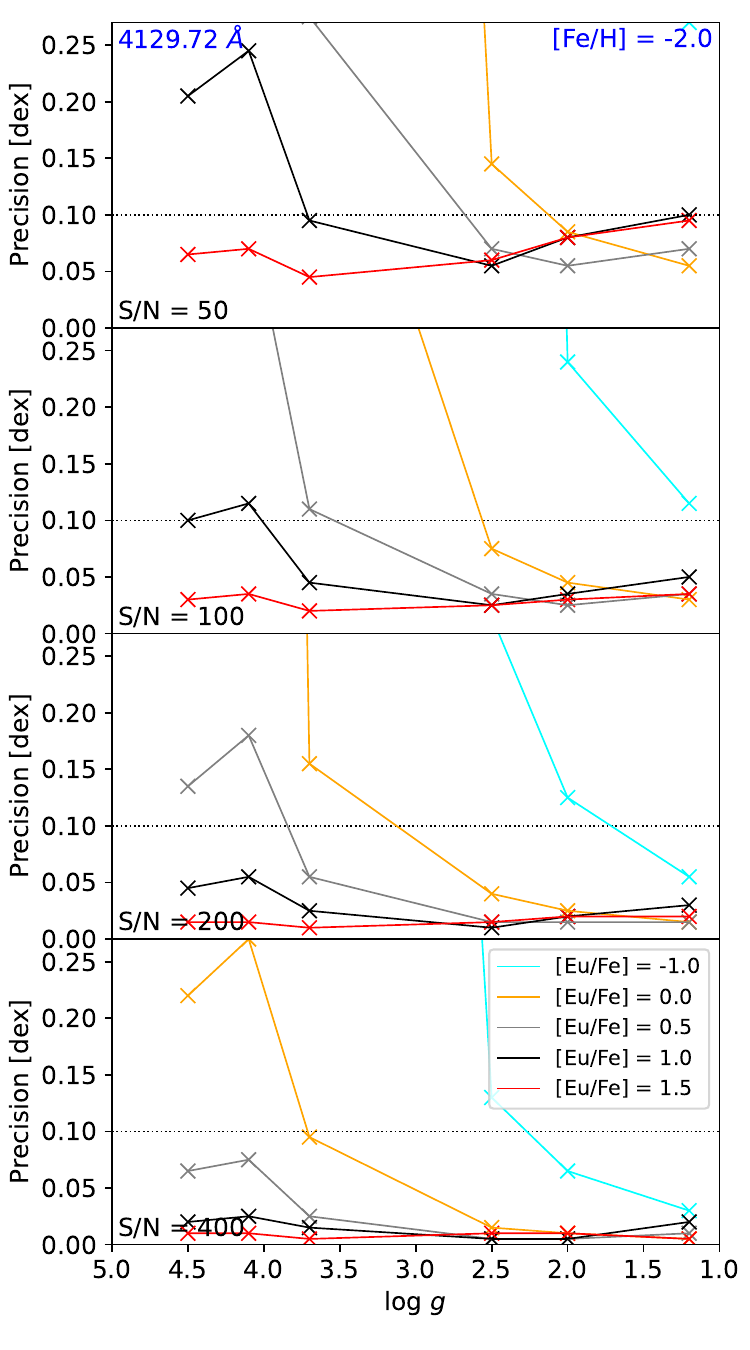} 
   \includegraphics[width=0.24\linewidth]{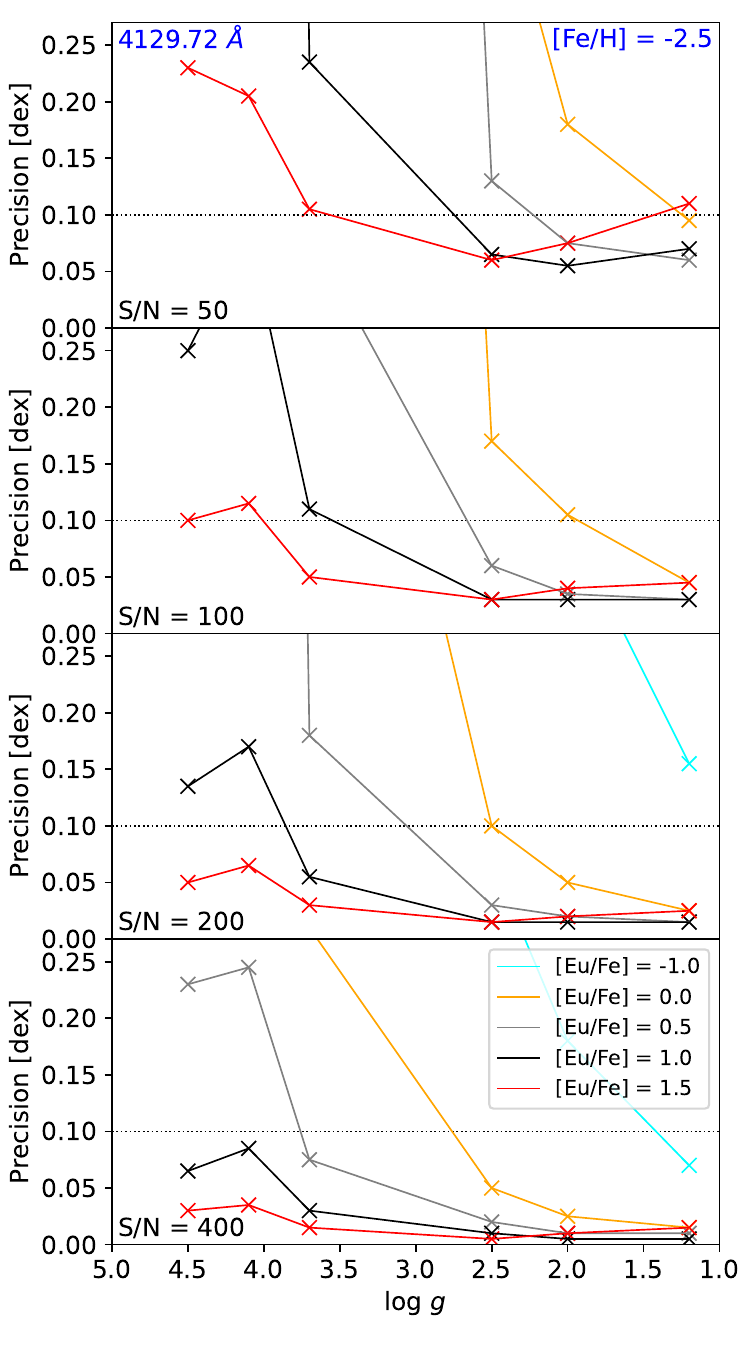}   
    \caption{Precision in the measurement of Eu abundances as a function of metallicity and of SNR. Stellar parameters are as in Fig.~\ref{fig:th_precision}. }
    \label{fig:origin_eu_precision}
\end{figure}

\begin{figure}
\centering
    \includegraphics[width=0.24\linewidth]{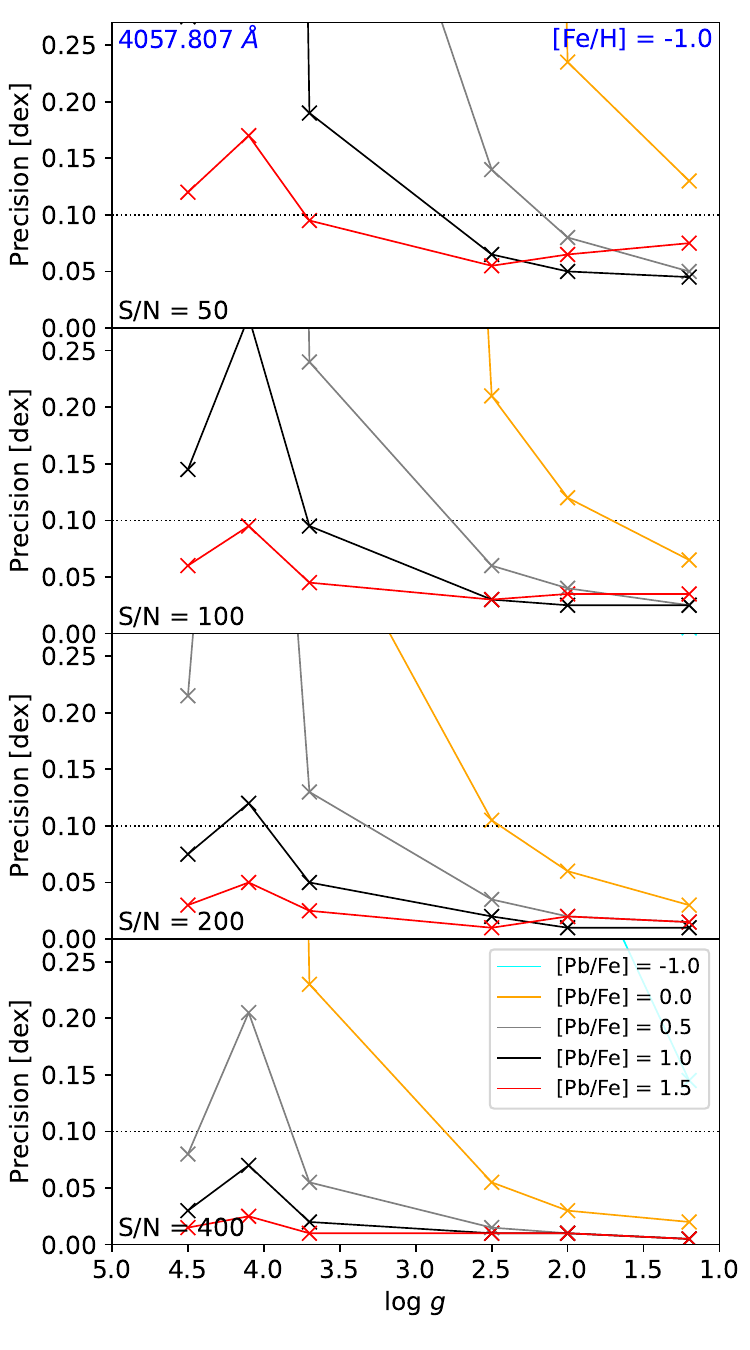} 
    \includegraphics[width=0.24\linewidth]{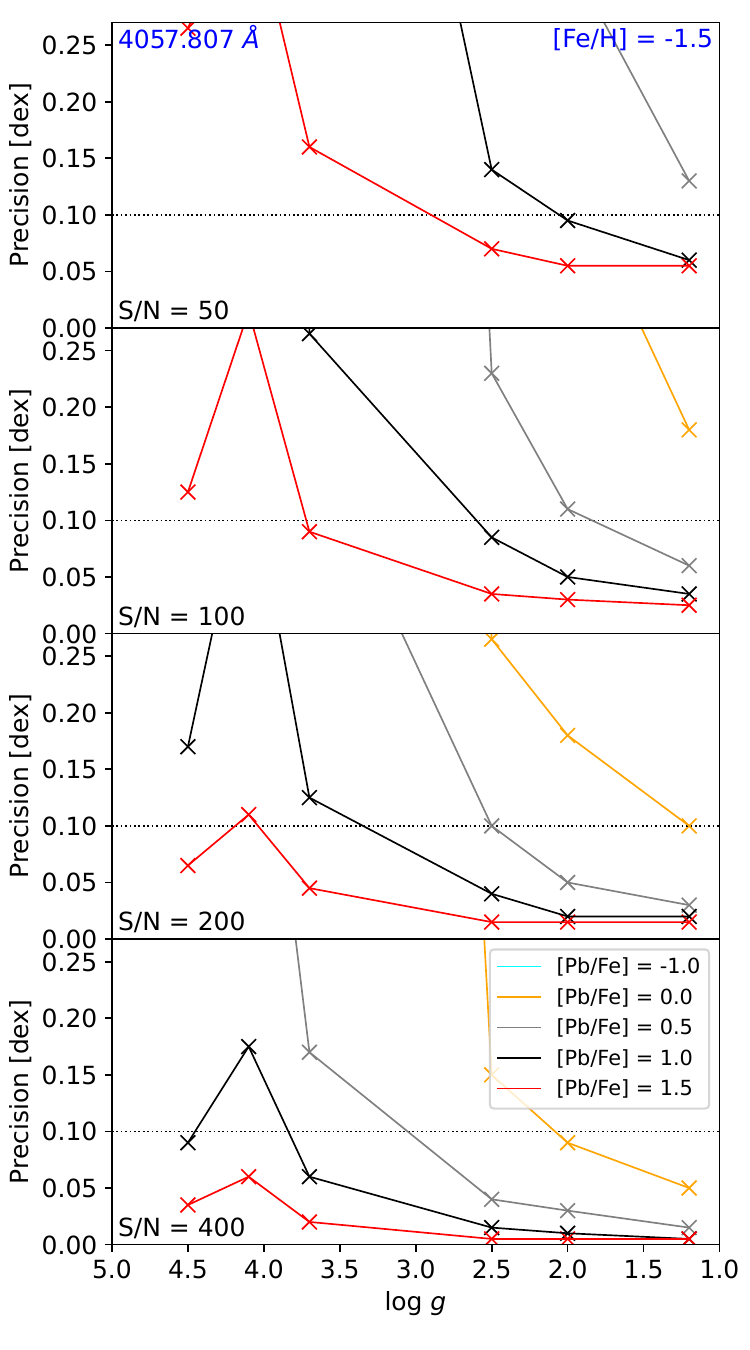} 
   \includegraphics[width=0.24\linewidth]{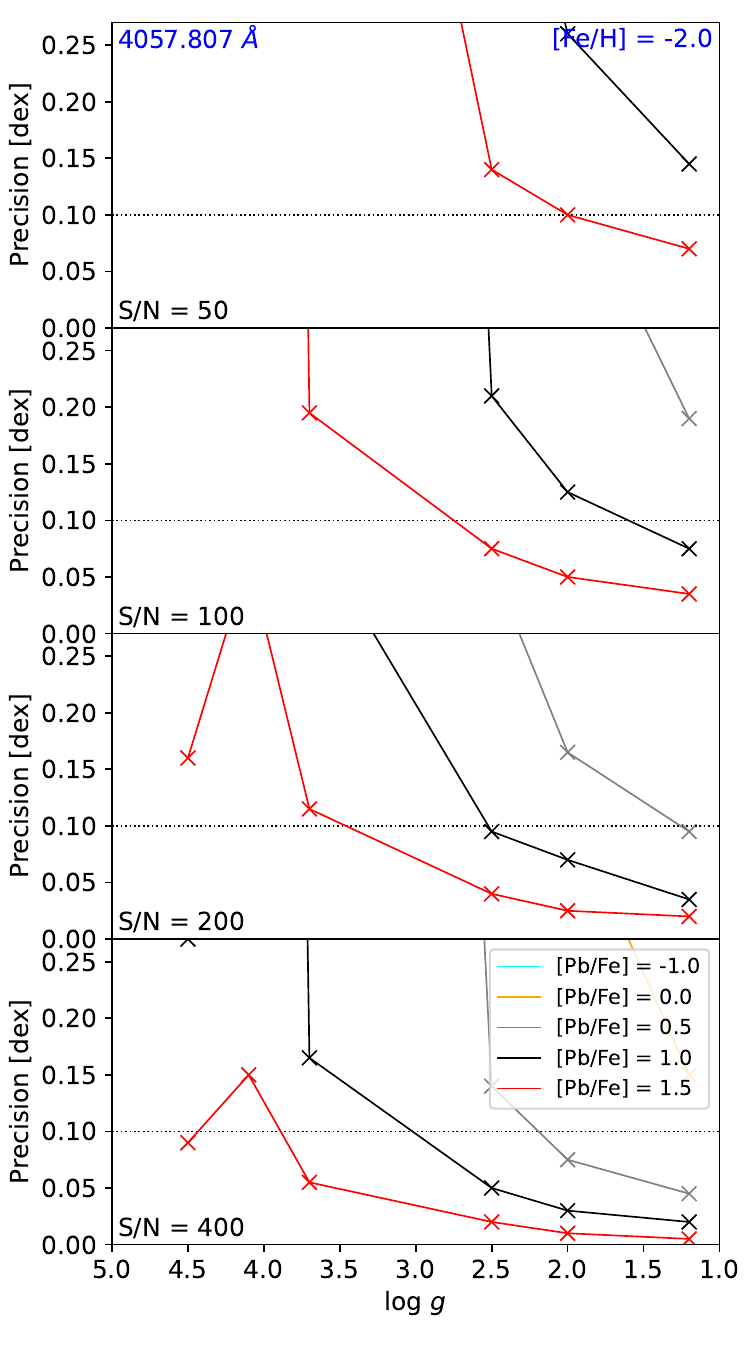} 
   \includegraphics[width=0.24\linewidth]{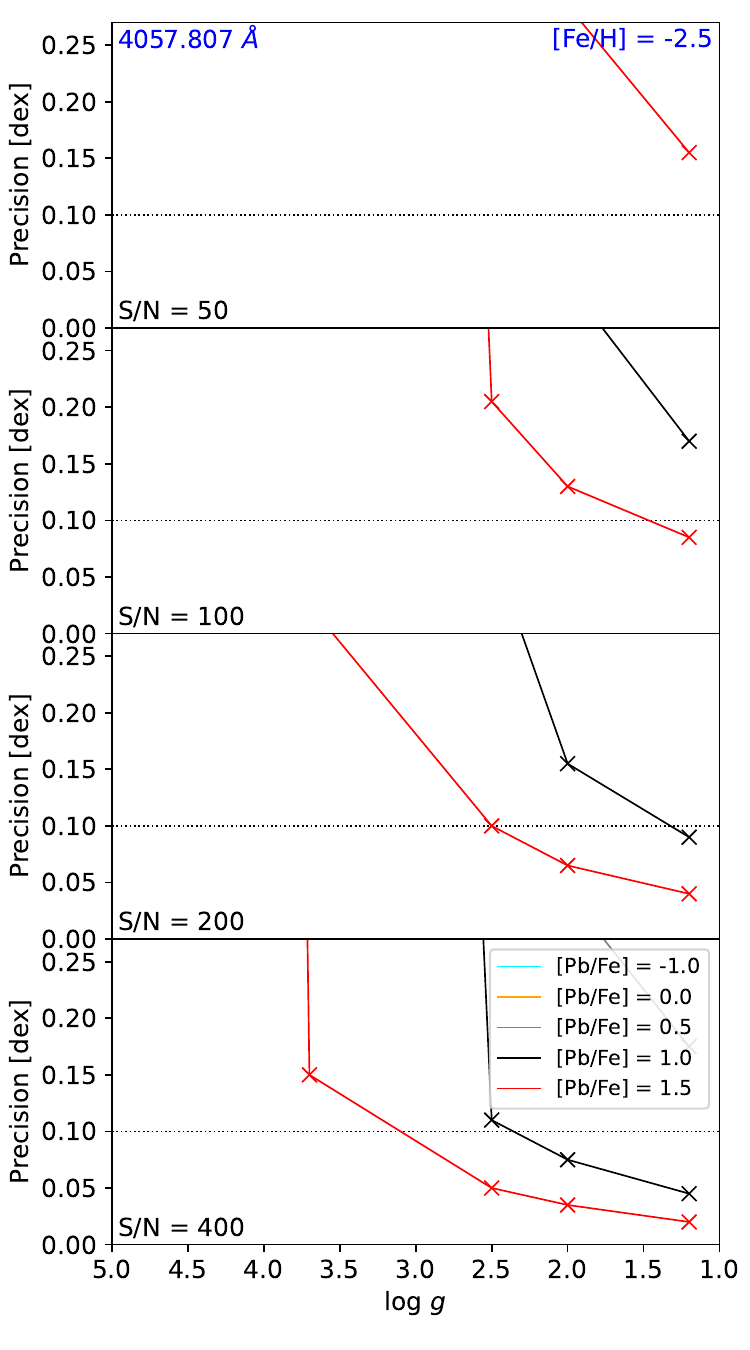}   
    \caption{Precision in the measurement of Pb abundances as a function of metallicity and of SNR. Stellar parameters are as in Fig.~\ref{fig:th_precision}. }
    \label{fig:origin_pb_precision}
\end{figure}

\begin{figure}
\centering
\includegraphics[width=0.24\linewidth]{precision_feh10.pdf} 
    \includegraphics[width=0.24\linewidth]{precision_feh15.pdf} 
   \includegraphics[width=0.24\linewidth]{precision_feh20.pdf} 
   \includegraphics[width=0.24\linewidth]{precision_feh25.pdf}   
    \caption{Precision in the measurement of Ba isotopic ratio as a function of metallicity and of SNR. Stellar parameters are as in Fig.~\ref{fig:th_precision}. }
    \label{fig:origin_ba_precision}
\end{figure}
